# Supplementary material for: Income and Poverty in a Developing Economy
Source: arXiv:0905.3803 source file (2009-05-25)
Supplement: Supplementary file 1 [file SM.pdf]

## SUPPLEMENTARY MATERIAL 1 ANALYTICAL SOLUTION OF THE FOKKER-PLANCK EQUATION

The starting equation is the Fokker-Planck equation:

$$\begin{aligned}\frac{\partial \hat{f}}{\partial t} &= \frac{\partial}{\partial y}\left([(M+2)y - c(t)]\hat{f} + y^2\frac{\partial \hat{f}}{\partial y}\right)\\ &= (M+2)\hat{f} + [(M+2)y - c(t)]\frac{\partial \hat{f}}{\partial y} + 2y\frac{\partial \hat{f}}{\partial y} + y^2\frac{\partial^2 \hat{f}}{\partial y^2}\\ &= y^2\frac{\partial^2 \hat{f}}{\partial y^2} + [(M+4)y - c(t)]\frac{\partial \hat{f}}{\partial y} + (M+2)\hat{f} \qquad (1)\end{aligned}$$

Let us consider a solution by separation of variables:

$$\hat{f}(y,t) = \sum_{n=0}^{n=\infty} a_n(t)\, g_n(y) \qquad (2)$$

Using eqn (2) in eqn (1), we get

$$\sum_{n=0}^{n=\infty} [\ \frac{y^2}{g_n(y)}\frac{\partial^2 g_n(y)}{\partial y^2} + \frac{[(M+4)y - c(t)]}{g_n(y)}\frac{\partial g_n(y)}{\partial y} + M + 2 - \frac{1}{a_n(t)}\frac{\partial a_n(t)}{\partial t}\ ]a_n(t)g_n(y) = 0 \qquad (3)$$

Eqn (3) above can be represented by two equations, as follows:

$$\frac{da_n(t)}{dt} = -\omega_n a_n(t) \ \Rightarrow\ a_n(t) \sim \exp[-\omega_n(t)] \qquad (4)$$

$$y^2\frac{d^2 g_n(y)}{dy^2} + [(M+4)y - c(t)]\frac{dg_n(y)}{dy} + (M+2-\omega_n)g_n(y) = 0 \qquad (5)$$

We can now solve eqn (5) and this gives a solution in terms of confluent hypergeometric functions $F(\alpha, \beta, c(t)/y)$.

$$\begin{aligned}g_n(y) &= A_1\,[\frac{c(t)}{y}]^{\alpha_-}\ F(\alpha_-, \beta_-, -\frac{c(t)}{y})\\ &+ A_2\,[\frac{c(t)}{y}]^{\alpha_+}\ F(\alpha_+, \beta_+, , -\frac{c(t)}{y}) \qquad (6)\end{aligned}$$

$$\alpha_\pm = \frac{3 + M \pm \sqrt{(1+M)^2 + 4\omega_n}}{2},$$

$$\beta_\pm = 1 \pm \sqrt{(1+M)^2 + 4\omega_n},$$

with $\omega_n = 2\pi n$ for periodic solutions and $A_i$ (i=1,2) are two arbitrary constants to be determined from initial conditions.

We note that one can use the method of Laplace transform (for two variables) in solving eqn (1) instead. The answer remains exactly the same.

### Confluent Hypergeometric Function

The confluent hypergeometric function has many representations. As a simple example, we define it through an identity

$$\int_0^\infty t^{\alpha-1}\, F(a,b,-t)\, dt = \frac{\Gamma(b)\,\Gamma(a-\alpha)\,\Gamma(\alpha)}{\Gamma(a)\,\Gamma(b-a)} \quad \text{for} \quad 0 < Re(\alpha) < Re(a) \qquad (7)$$

## SUPPLEMENTARY MATERIAL 2 TIME DEPENDENCE OF THE CPI AND POVERTY MEASURE

The $C_0$ parameter in our equation is fitted to the mean deflated income for each year, with the deflation taken from the independent CPI measure. The annual variation of this, used as a scaling parameter, is given in fig1.In order to extract the poverty index from our model, we need the deflated parameters $V(t)$ and $K(t)$. These are obtained from fitting to the cereal expenditure data from the NSS data, by extrapolating the real 'deflated' data set that we derived using a $\chi^2$ fitting method. Both theoretically formulae give excellent fits to the real data set. The time variation of these quantities is shown in fig.2.

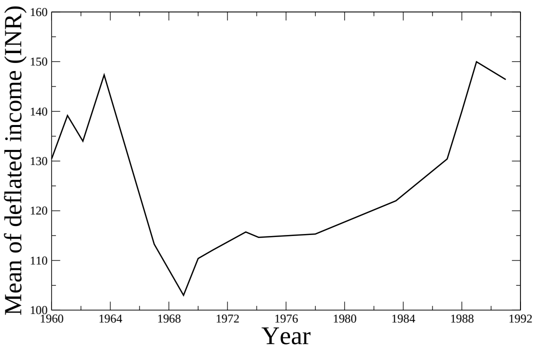


FIG. 1: Graph showing the variation of mean deflated income with time

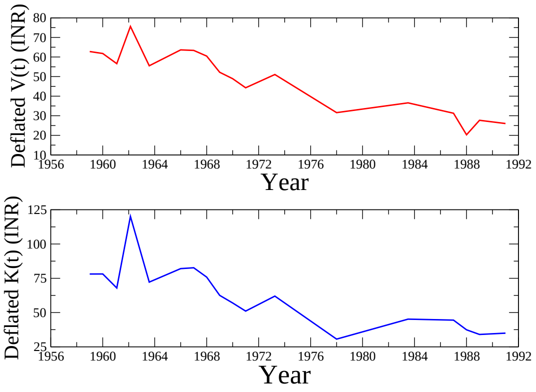


FIG. 2: Parameters V and K which relate the actual cereal consumption in the NSS to the deflated income, as defined by Eq.8 of the main text Parameter V is the maximum or saturation level of consumption in real terms, whereas K is the income required to purchase the V level of maximum consumption. Since both C and y are in defined real terms, K is also interpreted in real terms.
